# Supplementary material for: The Shapley Value of Classifiers in Ensemble Games
Source: arXiv:2101.02153 source file (2021-06-10)
Supplement: Supplementary file 1 [file appendix.tex]

\section{Model complexity and influence experimental details}\label{appendix:heterogeneity_experiment}
We extracted the Weisfeiler-Lehman features which appeared in at least 5 graphs in the datasets. We defined the frequency based graph descriptors used in Appendix \ref{appendix:model_selection}. The models were trained with 50\% of the dataset and the average Shapley values were calculated from the remaining 50\% of graphs.
\subsection{Neural network ensembles}
We created an ensemble of $m=10^3$ neural networks using \textit{scikit-learn} -- each of these had a single hidden layer. Each model received 20 randomly selected frequency features as input and had a randomly chosen number of hidden layer neurons -- we uniformly sampled this hyperparameter from $\left \{2^3, 2^4, 2^5, 2^6, 2^7\right\}$. Individual neural networks were trained by minimizing the binary cross-entropy with SGD for 200 epochs with a learning rate of $10^{-2}$. The results in Section \ref{sec:shapley_experiments} and the ones in Figure \ref{fig:shapley_twitch_neural} demonstrate that complexity (number of free parameters) is correlated with relative model importance.

\input{./figures/neural_net_twitch.tex}

\subsection{Random forest ensembles}
We created a random forest ensemble of $m=10^3$ classification trees using \textit{scikit-learn}. Each tree in the ensemble received 20 randomly selected Wesifeiler-Lehman count features as input. We used the default settings of \textit{scikit-learn} except for the maximal depth which we fixed to be 4. Using the Reddit and Twitch datasets we plotted on Figures \ref{fig:shapley_random_forest_complexity_1} and \ref{fig:shapley_random_forest_complexity_2} the mean normalized Shapley value of classification trees obtained by \textit{Troupe} in the ensemble games and dual ensemble games conditioned on the number of leaves that the trees have. 
\input{./figures/model_complexity_nice_bars_reddit.tex}

Our results support the claim made earlier that more complex models (higher number of tree leaves) contribute to correct and incorrect classification decisions with a higher probability. However, in this case the higher number of leaves might be a random artifact of sampling better quality features which are more discriminative.

\input{./figures/model_complexity_nice_bars_twitch.tex}
